# Supplementary material for: DiffAvatar: Simulation-Ready Garment Optimization with Differentiable Simulation
Source: arXiv:2311.12194 source file (2024-03-29)
Supplement: Supplementary file 2 [file Supplemental.tex]

% CVPR 2023 Paper Template
% based on the CVPR template provided by Ming-Ming Cheng (https://github.com/MCG-NKU/CVPR_Template)
% modified and extended by Stefan Roth (stefan.roth@NOSPAMtu-darmstadt.de)

\documentclass[10pt,twocolumn,letterpaper]{article}

%%%%%%%%% PAPER TYPE  - PLEASE UPDATE FOR FINAL VERSION
%\usepackage[review]{cvpr}      % To produce the REVIEW version
\usepackage{cvpr}              % To produce the CAMERA-READY version
%\usepackage[pagenumbers]{cvpr} % To force page numbers, e.g. for an arXiv version

% Include other packages here, before hyperref.
\usepackage{graphicx}
\usepackage{amsmath}
\usepackage{amssymb}
\usepackage{booktabs}

\usepackage{bm}
\usepackage{amsmath}
\usepackage{colortbl}
\usepackage[dvipsnames,svgnames]{xcolor}
\usepackage{blindtext}
\usepackage{lipsum,lineno}
\usepackage{multirow}
\usepackage{tikz}
\usepackage{wrapfig}
\usepackage{cases}
\usepackage{pifont}% http://ctan.org/pkg/pifont

% It is strongly recommended to use hyperref, especially for the review version.
% hyperref with option pagebackref eases the reviewers' job.
% Please disable hyperref *only* if you encounter grave issues, e.g. with the
% file validation for the camera-ready version.
%
% If you comment hyperref and then uncomment it, you should delete
% ReviewTempalte.aux before re-running LaTeX.
% (Or just hit 'q' on the first LaTeX run, let it finish, and you
%  should be clear).
\usepackage[pagebackref,breaklinks,colorlinks,bookmarks=false]{hyperref}

% Support for easy cross-referencing
\usepackage[capitalize]{cleveref}
\crefname{section}{Sec.}{Secs.}
\Crefname{section}{Section}{Sections}
\Crefname{table}{Table}{Tables}
\crefname{table}{Tab.}{Tabs.}

%%%%%%%%% PAPER ID  - PLEASE UPDATE
 % *** Enter the CVPR Paper ID here

\input{main/commands}
\begin{document}

\title{Supplementary Material \\ \papername : Simulation-Ready Garment Optimization with Differentiable Simulation}

\input{Supplementary/supplementary-content}

{\small
\bibliographystyle{ieee_fullname}
\bibliography{References}
}
\end{document}
